# Supplementary material for: Adapting Stochastic Search For Real-time Dynamic Weighted Constraint Satisfaction
Source: arXiv:1507.06045 source file (2015-07-22)
Supplement: Supplementary file 1 [file appendix.tex]

\chapter{Sample Appendix\label{appendix_notes}}
Here is some text in the sample appendix.
